# Supplementary material for: Harmony in Diversity: Merging Neural Networks with Canonical Correlation Analysis
Source: arXiv:2407.05385 source file (2024-07-07)
Supplement: Supplementary file 1 [file z0_additional_text.tex]

\section{Discussion}
Past works have focused almost exclusively on merging only pairs of models. While some papers discuss the possibility of merging multiple models, the proposed method is simply to apply the 2 model merging method iteratively to align all models to a single, reference model, and then to average all models. While this works to some extent in practice and is also what we do with CCA merging, it would be interesting to explore methods that are inherently made to merge multiple models all at once.

Our method is somewhat unsymmetric, merging model X to model Y destroys some of the information from model X. Despite this we perform better than the other methods we compare to.

\paragraph{Merging spaces} When the model architecture is such that the information flows sequentially from input layer to output layer, as is the case for MLPs or VGGs, a transformation needs to be computed after each layer. However, when the architecture is more complex, as is the case for ResNets for example, the transformations are not necessarily computed at each layer, rather they are computed whenever there is a change in the representation space. We refer to these specific points in a network as ``merging'' or ``alignment'' spaces. For example, blocks containing skip connections preserve the same representation space since the output space is forced to be consistent with the input one by the skip connections. The convolutional layers inside the block on the other hand can transform the representation spaces an therefore transformations need to be computed after those.

\paragraph{A note on merging in the common space}
Given that CCA naturally finds a space which maximally correlates the activations of both models being merged it is natural to think of merging the models in this common space. This would be done by transforming the parameters of model $\mathcal{A}$ with the found transformations $\{W_i^\mathcal{A}\}_{i=1}^{N-1}$ and transforming the parameters of model $\mathcal{B}$ with transformations $\{W_i^\mathcal{B}\}_{i=1}^{N-1}$ and then averaging the transformed parameters. We have tried this with no success. We hypothesize that the reason this way of merging fails is that the common representation space found by CCA is not fit to work with ReLU activation functions. The following paragraph provides a justification for this hypothesis.

For the pre-activations to remain informative after the application of ReLU, all the important information needs to be in the orthant (high-dimensional analog of the quadrant in the plane) of the pre-activation space corresponding to all variables having greater values than zero. That way important information is preserved by the ReLU function and only un-important information, which can be found in the other orthants with some variables having negative values, get squashed to 0. There is no inherent reason for the common space found by CCA to keep important information only in the positive orthant, rather it likely spreads it across all orthants. As the dimensionality of the space increases, the ratio between the volume of the positive orthant and the rest of the volume of the space decreases exponentially, in 1D the positive part of the line represents half of the space, in 2D the positive quadrant represents one quarter of the plane, in 3D the positive orthant represents one eighth of the space, etc. Therefore, given the typical high dimensionality of ANN embedding spaces it is probable that only a small fraction of the important information is kept in the positive orthant and thus preserved after applying the ReLU activation, on the other hand the rest of the information is getting at least partially squashed to 0.

\paragraph{Why CCA Merge destroys in part the model being aligned}
It is well known that artificial neural networks are invariant to permutations. Permuting the order of the neurons at a given layer equivalently permutes the pre-activations, the activations and any other commonly used operations in ANNs which are applied element-wise.
%
On the other hand, when considering linear combinations of features, as we do for CCA Merge, the weights of a given layer are combined as dictated by the found transformation $T$, recall the two equations:
\[x_i^\mathcal{B} = \sigma(T_iW_i^\mathcal{B}x_{i-1}^\mathcal{B}+T_ib^\mathcal{B}_i)\]
\[x_{i+1}^\mathcal{B} = \sigma(W_{i+1}^\mathcal{B}T_i^{-1}x_{i}^\mathcal{B}+b^\mathcal{B}_{i+1})\]
Since $T$ here linearly combines features and is not simply a change in the order of those features, applying a non-linear activation function element-wise will affect the activations themselves, which will no longer have the same numerical values as the un-transformed ones (albeit possibly in a different order). Therefore, when applying the inverse transformation $T^{-1}$ to these activations we are not able to reconstruct the exact representations of the original models.
Additionally, since the inverse transformation $T^{-1}$ is only applied at the level of the weights of the following layer, it receives the activations post activation function and no longer allows to retrieve the exact same.

Suppose we are trying to merge two models $\mathcal{A}$ and $\mathcal{B}$ so we align model $\mathcal{B}$ to model $\mathcal{A}$ by applying the found transformations at relevant layer. We denote the aligned model $\mathcal{B}$ by $\mathcal{B}'$, i.e. model $\mathcal{B}$ after applying all the transformations $\{T_i\}$ and their inverses $\{T^{-1}_i\}$ to the relevant layers. If the transformations are permutations, then $\mathcal{B}$ and $\mathcal{B}'$ are equivalent and represent the same mathematical function, modulo permutations of their internal representations. If on the other hand the transformations are not permutations, but rather linear combinations as it is the case for CCA Merge, then the two models are no longer equivalent. 

% \begin{table}[t]
% \caption{VGG11/CIFAR10-Logits whole dataset 2 models averaging accuracies}
% \label{t:resnet20_cifar100_none}
% \begin{center}
% \begin{tabular}{l|l l l l}
%             Widths & x1 & x2 & x4 & x8\\
%             \hline
%             Base models avg. & 87.24 $\pm$ 0.23\% & 87.44 $\pm$ 0.70 \% & 87.85 $\pm$ 0.25\% & 87.93 $\pm$ 0.50\%\\
%             Ensemble & 90.47 $\pm$ 0.12\% & 90.42 $\pm$ 0.22\% & 90.81 $\pm$ 0.09\% & 90.75 $\pm$ 0.20\%\\
%             \hline
%             Direct averaging & 10.00 $\pm$ 0.01\% & 10.00 $\pm$ 0.01\% & 10.00 $\pm$ 0.01\% & 10.00 $\pm$ 0.01\%\\
%             Permute & 15.44 $\pm$ 2.50\% & 16.73 $\pm$ 3.77\% & 24.55 $\pm$ 1.58\% & 19.99 $\pm$ 3.48\%\\
%             ZipIt! & 12.41 $\pm$ 2.60\% & - & - & - \\
%             \hline
%             \rowcolor{BrightGreen}
%             CCA & 80.23 $\pm$ 2.16\% & 78.14 $\pm$ 1.29\% & 84.44 $\pm$ 0.93\% & 82.38 $\pm$ 2.37\%\\
%         \end{tabular}
% \end{center}
% \end{table}

% [INTERPOLATION PLOTS, ONLY 2 SPLITS]

% [TABLES WITH RESULTS, ONLY 2 SPLITS]

% \begin{table}[t]
% \caption{ResNet20/CIFAR100 unbalanced subsets model averaging accuracies}
% \label{t:resnet20_cifar100_unbalanced}
% \begin{center}
% \begin{tabular}{l|l l l l}
%             Widths & x1 & x2 & x4 & x8\\
%             \hline
%             Base models & 52.61 $\pm$ 1.84\% & 56.78 $\pm$ 1.96 \% & 58.74 $\pm$ 1.93\% & 59.98 $\pm$ 1.80\%\\
%             Ensemble & 64.68 $\pm$ 0.76\% & 69.92 $\pm$ 0.75\% & 72.18 $\pm$ 0.67\% & 73.77 $\pm$ 0.44\%\\
%             \hline
%             Direct averaging & 1.48 $\pm$ 0.17\% & 3.12 $\pm$ 0.49\% & 7.03 $\pm$ 0.49\% & 20.55 $\pm$ 3.07\%\\
%             Permute & 20.66 $\pm$ 0.87\% & 39.05 $\pm$ 0.42\% & 51.55 $\pm$ 0.86\% & 58.45 $\pm$ 1.76\%\\
%             CCA & 24.46 $\pm$ 320\% & 44.59 $\pm$ 1.80\% & 55.61 $\pm$ 0.63\% & 60.38 $\pm$ 1.68\%\\
%         \end{tabular}
% \end{center}
% \end{table}

% \begin{table}[t]
% \caption{ResNet20/CIFAR100-CLIP whole dataset 5 models averaging accuracies}
% \label{t:resnet20_cifar100_none}
% \begin{center}
% \begin{tabular}{l|l l l l}
%             Widths & x1 & x2 & x4 & x8\\
%             \hline
%             Base models avg. & 69.19 $\pm$ 0.22\% & 74.06 $\pm$ 0.19 \% & 77.23 $\pm$ 0.32\% & 78.73 $\pm$ 0.24\%\\
%             Ensemble & 76.53 $\pm$ 0.14\% & 79.55 $\pm$ 0.11\% & 81.54 $\pm$ 0.05\% & 82.24 $\pm$ 0.16\%\\
%             \hline
%             Direct averaging & 1.02 $\pm$ 0.12\% & 1.06 $\pm$ 0.23\% & 1.27 $\pm$ 0.10\% & 1.46 $\pm$ 0.11\%\\
%             Permute & 17.01 $\pm$ 2.31\% & 32.18 $\pm$ 0.77\% & 51.81 $\pm$ 0.53\% & 65.25 $\pm$ 0.24\%\\
%             Git Re-Basin & - & 44.69 $\pm$ 1.04\% & 59.67 $\pm$ 0.32\% & 67.21 $\pm$ 0.14\%\\
%             Many Merge & - & 3.82 $\pm$ 0.66\% & 5.26 $\pm$ 0.44\% & 10.19 $\pm$ 0.53\%\\
%             ZipIt! & 14.51 $\pm$ 0.99\% & 33.68 $\pm$ 1.24\% & 50.93 $\pm$ 0.49\% & 62.89 $\pm$ 0.38\%\\
%             \hline
%             \rowcolor{BrightGreen}
%             CCA & 25.19 $\pm$ 0.63\% & 49.54 $\pm$ 0.46\% & 62.72 $\pm$ 1.01\% & 72.66 $\pm$ 0.14\%\\
%         \end{tabular}
% \end{center}
% \end{table}

% In Tables \ref{t:resnet20_cifar100_none} and \ref{t:resnet20_cifar100_unbalanced} we show our results for the ResNet20 models of different widths trained on the CIFAR100 whole dataset or on unbalanced splits of the datasets respectively. We can see that across all model widths and both data distribution scenarios aligning model features with CCA leads to a smaller loss in accuracy when averaging the two aligned models than using permutations. Directly averaging the weights of the models without any kind of feature matching transformations yields very poor results as expected.
% %
% These results suggest that indeed looking for one-to-one mappings between neurons might be too restrictive since it does not capture more complex interactions between features of different models. The performance of CCA merging here suggests that computations conducted by some neurons in one network might be distributed across multiple neurons in another model.
